# Supplementary material for: First measurement of massive virtual photon emission from N* baryon resonances
Source: arXiv:2205.15914 source file (2026-03-24)
Supplement: Supplementary file 1 [file HADES_supplementalMaterial.pdf]

# First measurement of massive virtual photon emission from $N^*$ baryon resonances

R. Abou Yassine et al. (HADES collaboration)

## Supplemental Material

### S1. COMBINATORIAL BACKGROUND SUBTRACTION

Details on the  $e^+$  and  $e^-$  reconstruction, the efficiency corrections and on the cuts applied to reject the conversion pairs can be found in [? ?]. The combinatorial background (CB) is estimated bin-by-bin using the geometrical average of the numbers of like-sign pairs.  $N_{CB} = 2 \times \sqrt{N_{e^+e^+} N_{e^-e^-}}$ . If for a given bin, only  $N_{e^+e^+}$  or  $N_{e^-e^-}$  is non zero, then the arithmetic average is used:  $N_{CB} = N_{e^+e^+} + N_{e^-e^-}$ . In Fig. ??a, the CB, shown as red triangles is compared to the correlated signal obtained after CB subtraction (black disks). It can be clearly observed that the contribution of the CB to the total  $e^+e^-$  yield is significant only around 120 MeV/ $c^2$ , where a strong signal due to double conversion of photons from  $\pi^0$  decay is visible. The very steep increase of CB in this region leads to a systematic error of 40%, while the subtraction of the CB has no influence on the  $e^+e^-$  yield above 140 MeV/ $c^2$ .

### S2. NORMALISATION OF MEASUREMENTS ON POLYETHYLENE AND CARBON

Both carbon and polyethylene targets were used in the experiment. As described in detail in [?], the calibration of the pion beam momentum distribution and the accurate normalization of the measurements on both targets is based on the analysis of the exclusive  $\pi^-p \rightarrow \pi^-p$ ,  $\pi^-p \rightarrow n\pi^+\pi^-$  and  $\pi^-p \rightarrow p\pi^-\pi^0$  reactions, where kinematic constraints can be exploited, together with the accurate knowledge of the elastic cross section. A  $\chi^2$  minimization procedure was developed to compare reconstructed events measured with the polyethylene target to a combination of simulated events for the  $\pi^-p \rightarrow \pi^-p$ ,  $\pi^-p \rightarrow n\pi^+\pi^-$ ,  $\pi^-p \rightarrow p\pi^-\pi^0$  reactions and of events measured on the carbon target. This procedure allowed to identify for polyethylene measurements events produced from  $\pi^- + p$  and  $\pi^- + C$

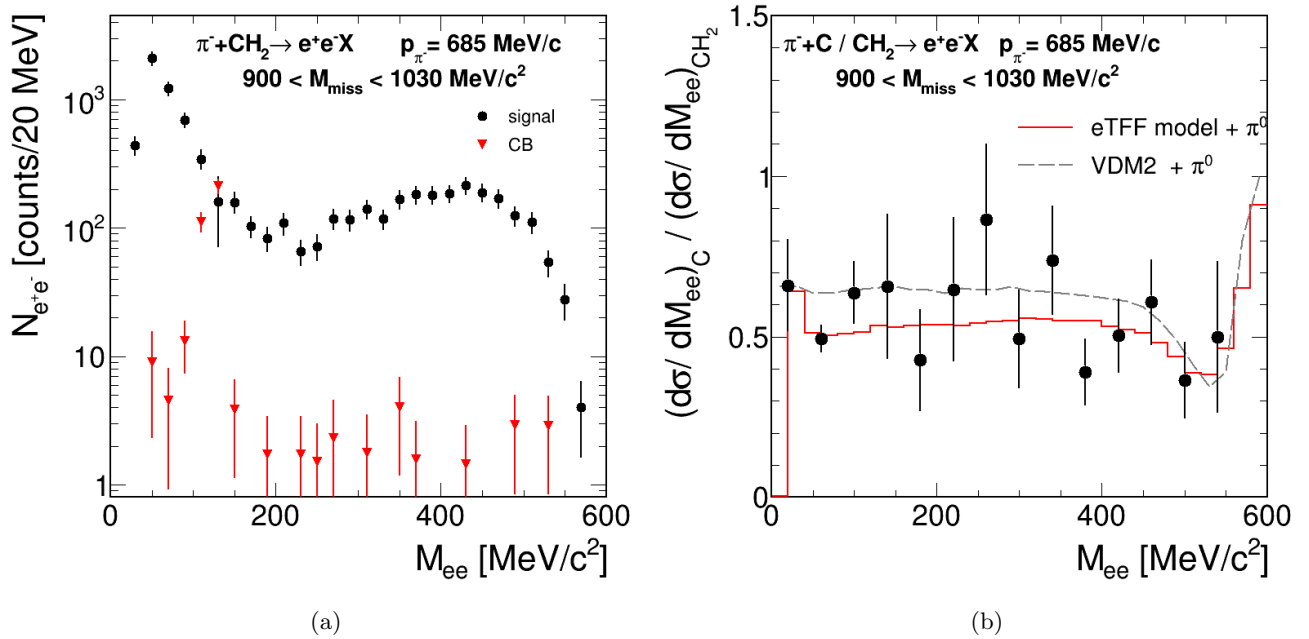

FIG. S1. (a) Efficiency corrected yields per 20 MeV wide bins as a function of the  $e^+e^-$  invariant mass. Full black disks and red triangles down display the correlated signal and the combinatorial background (CB), respectively. (b) The ratio of  $e^+e^-$  yields measured on the carbon and polyethylene targets for missing masses in the range [900-1030 MeV/ $c^2$ ] is shown as a function of  $M_{e^+e^-}$  as filled disks. The curves display the result of  $e^+e^-$  simulations for the eTFF (red curve) and VMD2 (dashed gray curve) models.

interactions, respectively. The relative normalization of measurements with the polyethylene and carbon targets was provided with a precision of 1% by comparing the yields from  $\pi^- + C$  reactions on both targets. On the other hand, the yield of elastic events from  $\pi^- + p$  interactions was compared to world data and SAID estimates for  $\pi^- p$  elastic scattering to deduce the normalization of the measurements on the polyethylene target and a precision of 4% could be obtained for the measurement at 0.685 GeV/c.

In Fig. 1 of the main text, differential cross sections integrated over the HADES acceptance for the  $\pi^- \text{CH}_2$ ,  $\pi^- + C$  and  $\pi^- p$  reactions are shown. A clear peak around the neutron mass is shown in all three cases, which is selected using a missing mass cut :  $900. < MM < 1030 \text{ MeV}/c^2$ . The differential cross sections resulting from the normalization of efficiency corrected yields after CB subtraction and after applying the missing mass selection are shown as black triangles up in Fig. 2a of the main text.

The ratio between the normalized yields measured on the carbon and polyethylene targets within the missing mass cut, which, as discussed below, is used to fix the ratio between the cross sections on carbon and proton is shown as a function of the invariant mass ( $M_{e^+e^-}$ ) in Fig. ??b.

### S3. SIMULATIONS OF THE $\pi^- p \rightarrow ne^+e^-$ REACTION

As the modelling of the  $\eta$  and  $\pi^0$  Dalitz decay, which are considered as a background in the present analysis, have been described in detail in [? ], we focus here on the contributions to the description of the  $\pi^- p \rightarrow ne^+e^-$  signal.

#### A. QED reference

The measured yields are first compared to the "QED reference" which derives from the  $\pi^- p \rightarrow n\gamma$  reaction in the limit of point-like baryons, *i.e.*, neglecting the  $q^2 = M_{e^+e^-}^2$  dependence of the eTFF. Assuming the formation of a baryon resonance (B) with a given spin and parity in the  $\pi^- p$  entrance channel, the differential cross sections for its Dalitz decay ( $B \rightarrow Ne^+e^-$ ) can be calculated exactly as a function of the invariant mass [? ]. As the PWA of both  $\gamma n$  and  $\pi\pi$  final states in the  $\pi^- p$  reaction indicate that the dominant resonant contributions are s-channel N(1520) ( $J^P=3/2^-$ ) and N(1535) ( $J^P=1/2^-$ ) [? ], the calculation was performed for these transitions. This leads to the same result for the partial decay width:

$$\Gamma_{QED}^{N^* \rightarrow N\gamma^*}(q^2) = \frac{\sigma_+^3 \sigma_-}{m_+^3 m_-} \times \Gamma^{N^* \rightarrow N\gamma}, \quad \text{where } m_{\pm} = m_{\star} \pm m_N \quad \text{and} \quad \sigma_{\pm}^2 = m_{\pm}^2 - M_{ee}^2. \quad (\text{S1})$$

$m_{\star}$  is the resonance mass and  $m_N$  the nucleon mass. Eq. (??), which directly relates the radiative and Dalitz decay widths, in the limit of point-like baryons, was then used for the generation of simulated events for the QED reference. The Dalitz differential decay width can then be calculated as a function of the  $e^+e^-$  invariant mass as :

$$\frac{d\Gamma_{QED}^{N^* \rightarrow Ne^+e^-}}{dM_{ee}} = \frac{2\alpha}{3\pi M_{ee}} \Gamma_{QED}^{N^* \rightarrow N\gamma^*}(M_{ee}), \quad (\text{S2})$$

Eq. (??) is strictly valid only for the contributions of the  $1/2^-$  and  $3/2^-$  partial waves to the  $\pi^- p \rightarrow ne^+e^-$  reaction. While interference effects between the contributions of various isospin will affect the total differential cross sections, it is however worth to be noted that other  $J^P$  configurations would lead to steeper distributions.

The integrated cross section for the  $\pi^- p \rightarrow ne^+e^-$  reaction is mostly sensitive to the differential cross section at small  $M_{e^+e^-}$  which does not depend on the  $J^P$  configuration. The Dalitz decay width at small  $M_{e^+e^-}$  can be approximated as:

$$\Gamma_{QED}^{N^* \rightarrow Ne^+e^-} \sim \frac{2\alpha}{3\pi} \Gamma^{N^* \rightarrow N\gamma} \log\left(\frac{m_-}{2m_e}\right) \quad (\text{S3})$$

where  $m_e=0.511 \text{ MeV}/c^2$  is the electron mass. For  $m^* \sim 1.49 \text{ GeV}/c^2$

$$\Gamma_{QED}^{N^* \rightarrow Ne^+e^-} \sim 1.34 \alpha \Gamma^{N^* \rightarrow N\gamma} \quad (\text{S4})$$

A similar relation can be derived for the cross sections

$$\sigma(\pi^- p \rightarrow Ne^+e^-) \sim 1.34 \alpha \sigma(\pi^- p \rightarrow N\gamma) \quad (\text{S5})$$

From the Bonn-Gatchina PWA, we have  $\sigma(\pi^- p \rightarrow N\gamma) = 220 \mu\text{b}$ , hence  $\sigma(\pi^- p \rightarrow Ne^+e^-) = 2.1 \mu\text{b}$ .

Taking into account this cross section value and Eq.(??) for the differential distribution as a function of  $M_{e^+e^-}$ , a well defined reference is obtained, which is in agreement with measurements of the  $\pi^- p \rightarrow n\gamma$  cross section.

## B. VMD models

To take into account the effect of eTFF, first VMD models are scrutinized. They are based on a two-step calculation, where, as described below, the  $\rho$  production step is adjusted to describe the results of the two-pion production analysis measured by HADES in the  $\pi^-p$  reaction at the same energy [?] and, in a second step, the  $\rho \rightarrow e^+e^-$  decay is treated in two options, following the VMD1 and VMD2 models.

### 1. $\rho$ spectral function and partial decay widths

Simulations of the  $\pi^-p \rightarrow ne^+e^-$  and  $\pi^-p \rightarrow n\pi^+\pi^-$  were performed using a modified version of the Pluto event generator [?]. The  $\rho$  meson spectral function has the form

$$\mathcal{A}(M) = \frac{M^2 \Gamma_{tot}(M)}{(M_\rho^2 - M^2)^2 + M^2 \Gamma_{tot}^2(M)}, \quad (\text{S6})$$

where  $M$  is the  $\rho$  mass and  $M_\rho$  its pole value. The total width  $\Gamma_{tot}(M)$  is the sum of the  $\rho \rightarrow \pi^+\pi^-$  and  $\rho \rightarrow e^+e^-$  partial decay widths.

$$\Gamma_{tot}(M) = \Gamma_{\pi^+\pi^-}(M) + \Gamma_{e^+e^-}(M) \quad (\text{S7})$$

The spectral function, as defined in Eq. (??) derives from the relation between the total width and the imaginary part of the self-energy  $\Sigma_\rho(M)$ :

$$\text{Im}(\Sigma_\rho(M)) = M \Gamma_{tot}(M). \quad (\text{S8})$$

To be consistent with the Bonn-Gatchina PWA approach, we used the following expressions of the decay widths :

$$\Gamma_{\pi^+\pi^-}(M) = \left(\frac{M_\rho}{M}\right)^2 \left(\frac{q_{\pi\pi}}{q_{0,\pi\pi}}\right)^3 \frac{1 + R^2 q_{0,\pi\pi}}{1 + R^2 q_{\pi\pi}}, \quad (\text{S9})$$

where  $q_{\pi\pi} = \frac{1}{2}(M^2 - 4m_\pi^2)^{1/2}$  is the center-of-mass momentum for the decay of the  $\rho$  meson into two pions, and  $q_{0,\pi\pi}$  the value for  $M=M_\rho$ .  $R=0.8$  fm is the cut-off parameter. Eq. (??) is similar to the Manley parameterization, commonly used in transport approaches, which however uses a softer cut-off value of 1 fm. For the  $\rho \rightarrow e^+e^-$  decay, we use the VMD1 and VMD2 models, as defined in [?], which are based on two different Lagrangians for the  $\gamma - \rho$  coupling. The respective partial decay widths are given by

$$\text{VMD1} : \Gamma(M_{e^+e^-})_{VMD1} = \Gamma_0 M_{e^+e^-} / M_0 \quad (\text{S10})$$

$$\text{VMD2} : \Gamma(M_{e^+e^-})_{VMD2} = \Gamma_0 (M_0 / M_{e^+e^-})^3, \quad (\text{S11})$$

respectively.

We wish to stress that these expressions of partial widths derive from the choice of total width definition. If the relation  $\text{Im}(\Sigma_\rho) = M_\rho \Gamma_{tot}(M)$  is used instead of Eq. (??), then the spectral function reads:

$$\mathcal{A}(M) = \frac{M_\rho^2 \Gamma_{tot}(M)}{(M_\rho^2 - M^2)^2 + M_\rho^2 \Gamma_{tot}^2(M)}, \quad (\text{S12})$$

and the expressions of the partial decay widths differ by a factor  $M/M_\rho$  w.r.t. Eqs. ??, ?? and ??.

### 2. $\rho$ production

A realistic description of the  $\rho n$  production differential cross sections in the  $\pi^-p$  reaction is essential for a consistent prediction of the  $\pi^-p \rightarrow ne^+e^-$  yields. This can be realized by using the  $\rho$  contribution obtained in the PWA for the  $\pi^-p \rightarrow n\pi^+\pi^-$  reaction at the same energy [?]. The corresponding differential cross section as a function of the  $\pi^+\pi^-$  invariant mass is displayed as black dots in Fig. ??a, where the errors represent the experimental uncertainties.

Simulations of the  $\pi^-p \rightarrow n\rho [\pi^+\pi^-]$  process were performed using the spectral function of Eq. (??) and the  $\rho \rightarrow \pi^+\pi^-$  partial width of Eq. (??). For the calculation of the total width, the  $\rho \rightarrow e^+e^-$  partial decay width was chosen following the VMD2 model (Eq.(??)). This choice has however an influence on the  $\pi^+\pi^-$  production channel only very close to the  $\pi^+\pi^-$  production threshold. The s-wave production of the  $\rho$  meson was simulated using phase

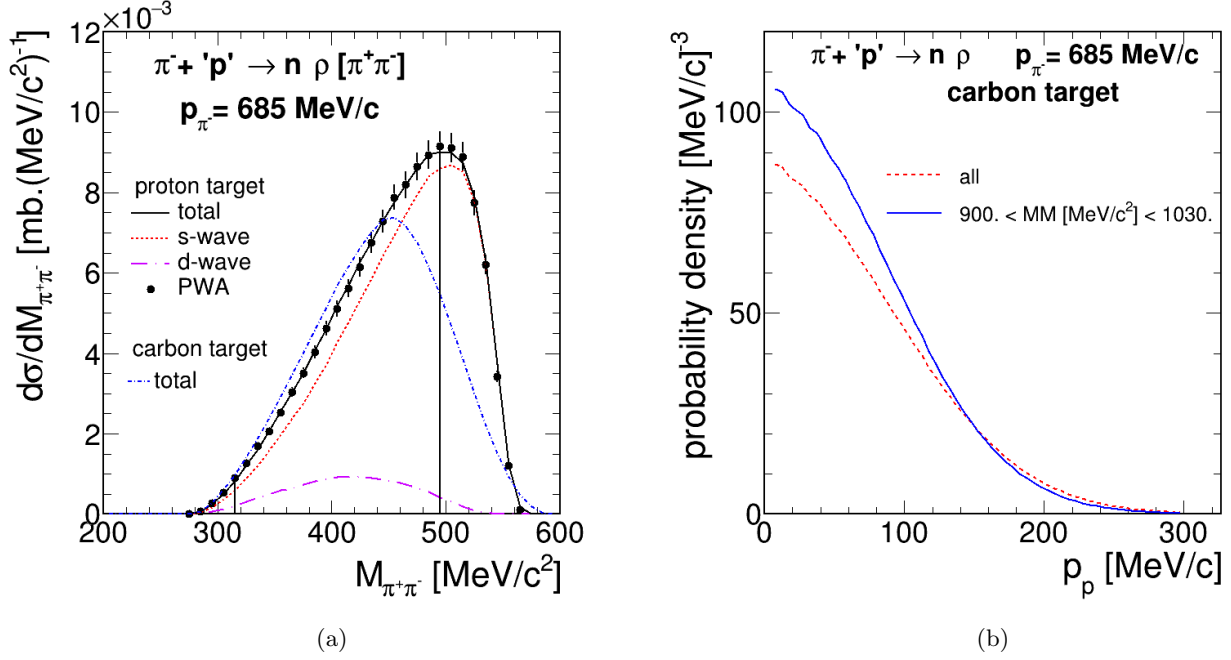

FIG. S2. (a) Full disks show the invariant mass distribution for  $\rho$  contribution in the PWA of the  $\pi^-p \rightarrow n\pi^+\pi^-$  with experimental systematic error bars [? ]. The curves display the result of a fit using simulated distributions for s- and d-wave  $\rho$ -n production (s-wave : short dashed red, d-wave: violet dash-dotted, sum: full black curve), which is used for the simulation of the  $\pi^-p \rightarrow n\rho$  reaction. The vertical lines show the range of invariant mass used for the fit. The dot-dashed blue line displays the result of the simulation for the  $\pi^-+C$  case, where the same  $\rho$  production cross section as for the  $\pi^- + p$  reaction is used and the missing mass cut  $900. < MM [\text{MeV}/c^2] < 1030.$  is applied. (b) The density probability distribution of the proton momentum in the carbon nucleus is shown with (full curve) and without (dashed curve) the cut on the missing mass in the  $\pi^-p \rightarrow \rho X$  reaction ( $900 < MM < 1030 \text{ MeV}/c^2$ ).

space distributions and, for the d-wave production, events were further weighted by a factor  $p_{CM}^2$ , where  $p_{CM}$  is the  $\rho$  center-of-mass momentum in the  $\pi^-p \rightarrow \rho n$  reaction. The resulting invariant mass distributions were used to determine the relative contribution of d-wave (pink curve) to s-wave (red curve) production by a fit to the PWA solution, as shown in Fig. ??a. The fit was performed in the range of invariant masses  $[320, 490 \text{ MeV}/c^2]$  in order to limit the sensitivity to resolution effects or to the incident pion beam momentum distribution. The best agreement with the PWA solution is obtained with a  $10 \pm 2\%$  d-wave contribution.

### 3. $e^+e^-$ distributions

The same  $\rho$  production model was used to generate  $e^+e^-$  events from the  $\rho$  decay, which is treated, using either the VMD1 or VMD2 partial decay widths, given in Eqs (??) and (??), respectively. The VMD2 model or "strict VMD" provides by itself a description of the full  $\pi^-p \rightarrow n e^+e^-$  process. In the case of VMD1, the vanishing  $\rho \rightarrow e^+e^-$  partial decay width for  $M_{e^+e^-}$  close to 0 is compensated by adding a contribution corresponding to the coupling of the real photon to point-like baryons, which is a salient feature of VDM1 [? ? ]. The latter is given by the QED reference introduced above. As the phase between the  $\rho$  and  $\gamma$  amplitudes is unknown, yields generated with the VMD1  $\rho$  decay model and with the QED reference models, respectively, were added using either a constructive or destructive interference contribution.

## S4. MODELLING OF QUASI-FREE $\pi^- + p$ REACTIONS IN THE CARBON NUCLEUS

To describe the  $e^+e^-$  production from the polyethylene target, interactions with carbon nuclei were treated in the simulation using a quasi-free participant spectator model. The  $^{12}\text{C}$  nucleus is represented as a spectator on-shell  $^{11}\text{B}$  and a participant off-shell proton. The proton momentum distribution is taken according to quasi-free  $^{12}\text{C}(e, e'p)$  measurements [? ]. As shown in Fig. ?? (right panel), the missing mass cut which is applied in the analysis (see

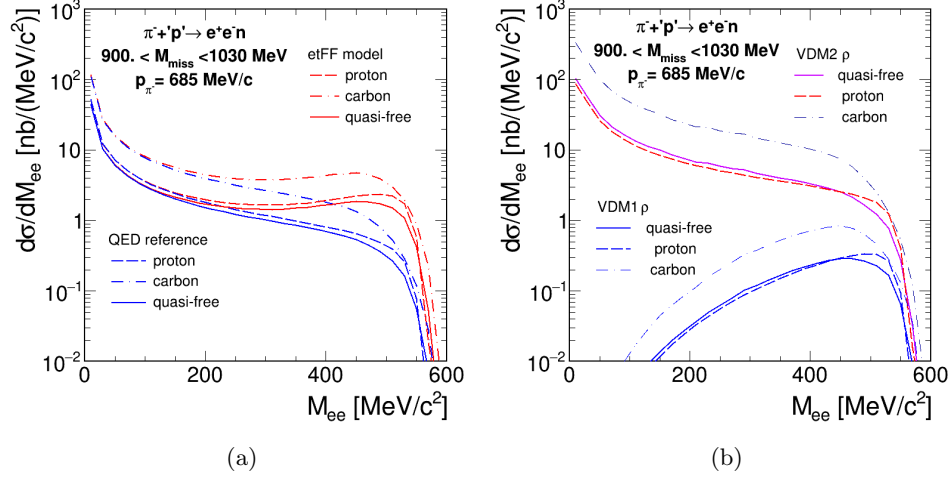

FIG. S3. (a) Differential cross sections as a function of the  $e^+e^-$  invariant mass in the simulations of baryon Dalitz decay in the  $\pi^-p$  (long dashed line) and  $\pi^- + C$  (dash-dotted line) reactions. Quasi-free reactions are selected by applying the cut  $900 < M_{miss} < 1030 \text{ MeV}/c^2$ , which affects only  $\pi^- + C$  interactions. The differential cross sections for the quasi-free reaction are obtained after dividing the  $\pi^- + CH_2$  curve by  $R_{CH_2/H} = 4.9$ . The red curves correspond to the eTFF model and the blue curves display the QED reference. (b) Same as (a) but for the VDM2 (pink curves) and VDM1 (blue curves).

Fig. 1 of the main text) reduces the sensitivity of the results to the high proton momentum tail of the distribution used in the simulation. As it can be observed in Fig. ??a, the  $\rho$  mass distribution for the production on carbon is significantly shifted towards lower values w.r.t. the proton target. This is due to the different phase space for the  $\rho$  meson production induced by the Fermi momentum in the participant spectator model. The  $\pi^0$ ,  $\rho$  and real photon production cross sections for interactions of  $\pi^-$  on the carbon nuclei were deduced from the free cross sections, using a constant factor  $R_{C/H} = \sigma_C/\sigma_H$ . For the  $\eta$  production, the steep increase of the cross section as a function of the energy above the production threshold is taken into account within the participant-spectator model, which results in an average cross section for the carbon target of the same order than for the proton target (see [?] for details).

Differential cross sections on the polyethylene targets are deduced from the corresponding proton and carbon ones:

$$\left(\frac{d\sigma}{dM_{ee}}\right)_{CH_2} = \left(\frac{d\sigma}{dM_{ee}}\right)_C + 2\left(\frac{d\sigma}{dM_{ee}}\right)_H. \quad (\text{S13})$$

To deduce from the  $CH_2$  measurements a cross section comparable to a free cross section, we define a "quasi-free" cross section as:

$$\left(\frac{d\sigma}{dM_{ee}}\right)_{qf} = \left(\frac{d\sigma}{dM_{ee}}\right)_{CH_2} / R_{CH_2/H}, \quad (\text{S14})$$

with

$$R_{CH_2/H} = 2 + R_{C/H}. \quad (\text{S15})$$

One can also introduce

$$R_{C/CH_2} = \frac{R_{C/H}}{2 + R_{C/H}}. \quad (\text{S16})$$

A ratio  $R_{C/H} = 2.9$  ( $R_{CH_2/H} = 4.9$  and  $R_C/CH_2 = 0.59$ ) has been chosen for the simulations of the  $\pi^- + C$  interactions. As shown in Fig. ??b, it allows for a consistent description of the ratio between the normalized differential yields measured on the carbon and polyethylene targets as a function of the invariant mass. This ratio stays close to the value  $R_C/CH_2 = 0.59$  in the whole invariant mass range.  $R_{C/H}$  can be interpreted as the number  $Z_{eff} = R_{C/H}$  of effective protons in the quasi-free  $\pi^- + C$  reaction. We estimate an error of  $\pm 0.5$  on this number, hence  $Z_{eff} = 2.9 \pm 0.5$ , which is consistent with a reaction with protons at the nuclear surface, where  $Z_{eff} = 6^{2/3} = 3.3$ . The ratios of the differential yields for the QED and eTFF models on the one hand and for all VMD models on the other hand are very

similar, so only the results of the eTFF and VMD2 models are shown in Fig. ??b. For the QED and eTFF models, the ratio directly derives from  $R_{C/H}$ . The small invariant mass dependence of the ratio of simulated yields on carbon and polyethylene targets is due to the effect of the Fermi motion and of the missing mass cut, which distorts the  $M_{e^+e^-}$  distribution measured on the carbon target. For the VMD models, the  $\rho$  mass distribution is shifted towards lower masses w.r.t. the free case, which results in a higher  $e^+e^-$  yield on the carbon target, for a given  $\rho$  production cross section.

The effect of the Fermi momentum on the  $e^+e^-$  yield is shown in more detail in fig. ?. Here, the differential cross sections for the proton, carbon and for the quasi-free process are shown for the eTFF model and the QED reference in panel a) and for the VMD1 and VMD2 models in panels (b), using the same missing mass cut ( $900. < M_{miss} < 1030$  MeV/ $c^2$ ) as applied for experimental data. The quasi-free curves are used for the comparison with data normalized for the quasi-free process, as shown in Fig. 2b and 2c of the main text.

- 
- [S1] F. Scozzi, *Studying excited states of the nucleon with the HADES detector at GSI*, PHD, Paris-Sud and TU Darmstadt universities, 2018.
  - [S2] P. Rodriguez-Ramos, Experimental results in pion induced reaction with carbon and polyethylene targets obtained by HADES-GSI, PHD, Czech Technical University in Prague, 2021.
  - [S3] J. Adamczewski-Musch *et al.*, Phys. Rev. **C102**, 024001 (2020), *Two-Pion production in the second resonance region in  $\pi^-p$  collisions with HADES*.
  - [S4] B. Ramstein, EPJ Web Conf. **241**, 01012 (2020), *Studying time-like electromagnetic baryonic transitions with HADES in pion induced reactions*.
  - [S5] M. I. Krivoruchenko, B. V. Martemyanov, A. Faessler, and C. Fuchs, Annals Phys. **296**, 299 (2002), *Electromagnetic transition form factors and dilepton decay rates of nucleon resonances*.
  - [S6] I. Fröhlich *et al.*, PoS **ACAT2007**, 076 (2007), *Pluto: A Monte Carlo Simulation Tool for Hadronic Physics*.
  - [S7] H. B. O'Connell, B. C. Pearce, A. W. Thomas, and A. G. Williams, Prog. Part. Nucl. Phys. **39**, 201 (1997),  *$\rho-\omega$  mixing, vector meson dominance and the pion form-factor*.
  - [S8] M. Zetenyi and G. Wolf, Phys. Rev. **C86**, 065209 (2012), *Dilepton production in pion-nucleon collisions in an effective field theory approach*.
  - [S9] B. Friman and H. J. Pirner, Nucl. Phys. **A617**, 496 (1997), *P wave polarization of the rho meson and the dilepton spectrum in dense matter*.
  - [S10] K. Nakamura, S. Hiramatsu, T. Kamae, H. Muramatsu, N. Izutsu, and Y. Watase, Nucl. Phys. A **268**, 381 (1976), *The Reaction C-12 ( $e, e'p$ ) at 700-MeV and DWIA Analysis*.
